# Supplementary material for: Generalizing Dataset Distillation via Deep Generative Prior
Source: arXiv:2305.01649 source file (2023-05-03)
Supplement: Supplementary file 1 [file _supplementary.tex]

\input{_constants}
\cameraready

\documentclass[10pt,twocolumn,letterpaper]{article}
\input{cvpr_header}
\myexternaldocument{_main}
\begin{document}
\title{\paperTitle \\ Supplemental Material}
\author{\authorBlock}
\maketitle

\input{12_appendix}

{\small
\bibliographystyle{ieee_fullname}
\bibliography{11_references}
}

\end{document}
